# Supplementary material for: Knowledge Graph Embeddings in Geometric Algebras
Source: arXiv:2010.00989 source file (2021-03-22)
Supplement: Supplementary file 1 [file appendix.tex]

\newpage
\begin{appendices}
\section{Supported Vector Space for GeomE}

\begin{table}[h!]%{r}{6.9cm}
\centering
\vspace{-1pt}
\caption{Supported Vector Space.}\label{wrap-tab:1}
%\begin{tabular}{lccccc}\\\toprule  
\begin{tabular}{
p{6cm}p{1.1cm}p{1.4cm}p{1.7cm}p{1.7cm}p{1.5cm} }\hline
         Models   & Real $\mathbb{R}$ & Complex $\mathbb{C}$ & Quaternion $\mathbb{H}$ & Octonion $\mathbb{O}$ &  n-grade $\mathbb{G}^n$ \\ \hline
TransE~\cite{TransE}           &  \checkmark    &   \xmark  & \xmark &  \xmark &  \xmark \\ 
DistMult~\cite{DISTMULT}           &  \checkmark    &   \xmark  & \xmark &  \xmark &  \xmark \\ 
TuckEr~\cite{Tucker}    &  \checkmark    &   \xmark  & \xmark &  \xmark &  \xmark \\ 
\hline
(p)RotatE~\cite{RotatE}            &   \checkmark    & \checkmark &  \xmark & \xmark & \xmark \\ 
ComplEx~\cite{ComplEx}                &\checkmark  & \checkmark  & \xmark   & \xmark & \xmark \\
TransComplEx~\cite{TransComplex}                &\checkmark  & \checkmark  & \xmark   & \xmark & \xmark \\
\hline
QuatE~\cite{QuatE}            &   \checkmark   & \checkmark  &  \checkmark &  \xmark   & \xmark \\ 
OctonionE~\cite{QuatE}   &   \checkmark   & \checkmark  &  \checkmark &  \checkmark   & \xmark \\ 
\hline
\hline
GeomE  & \checkmark & \checkmark  & \checkmark &  \checkmark &   \checkmark \\ \hline
\end{tabular}
\vspace{-10pt}
\label{table:trans}
\end{table}
\section{The Geometric Product of 3-grade Multivectors}~\label{3-grade product}
The product of two 3-grade multivectors 
$M_a = a_{0}+a_{1}e_{1}+a_{2}e_{2}+a_{3}e_{3}+a_{12}e_{1}e_{2}+a_{23}e_{2}e_{3}+a_{13}e_{1}e_{3}+a_{123}e_{1}e_{2}e_{3}$
and 
$M_{b}= b_{0}+b_{1}e_{1}+b_{2}e_{2}+b_{3}e_{3}+b_{12}e_{1}e_{2}+b_{23}e_{2}e_{3}+b_{13}e_{1}e_{3}+b_{123}e_{1}e_{2}e_{3}$ from $\mathbb{G}^3$ is represented as follows.

\begin{equation}
\begin{split}
M_{a} \otimes_3 M_{b} =& a_{0} b_{0}+a_{1} b_{1} + a_{2} b_{2} + a_{3} b_{3}-a_{12} b_{12}-a_{23} b_{23} - a_{13} b_{13} - a_{123} b_{123}\\
&+ (a_{0} b_{1} + a_{1} b_{0}-a_{2} b_{12} + a_{12} b_{2} - a_{3} b_{13} + a_{13} b_{3} - a_{23} b_{123} - a_{123} b_{23}) e_{1}\\
&+ (a_{0} b_{2} + a_{2} b_{0} + a_{1} b_{12} - a_{12} b_{1} - a_{3} b_{23} + a_{23} b_{3} + a_{13} b_{123} + a_{123} b_{13}) e_{2}\\
&+ (a_{0} b_{3} + a_{3} b_{0} + a_{1} b_{13} - a_{13} b_{1} + a_{2} b_{23} - a_{23} b_{2} - a_{12} b_{123} - a_{123} b_{12}) e_{3}\\
&+ (a_{0} b_{12} + a_{12} b_{0} + a_{1} b_{2} - a_{2} b_{1} - a_{13} b_{23} + a_{23} b_{13} + a_{3} b_{123} + a_{123} b_{3}) e_{1}e_{2}\\
&+ (a_{0} b_{23} + a_{23} b_{0} + a_{1} b_{123} + a_{123} b_{1} + a_{2} b_{3} - a_{3} b_{2} - a_{12} b_{13} + a_{13} b_{12}) e_{2}e_{3} \\
&+ (a_{0} b_{13} + a_{13} b_{0} + a_{1} b_{3} - a_{3} b_{1} - a_{2} b_{123} - a_{123} b_{2} + a_{12} b_{23} - a_{23} b_{12}) e_{1}e_{3}\\
&+ (a_{0} b_{123} + a_{123} b_{0} + a_{1} b_{23} + a_{23} b_{1} - a_{2} b_{13} - a_{13} b_{2} + a_{3} b_{12} + a_{12} b_{3}) e_{1}e_{2}e_{3}.
\end{split}
\vspace{-0.3cm} 
\end{equation}
\section{Extended Score Function of GeomE}~\label{extended scorefunction}
More specifically, we define the scoring functions for GeomE2D and GeomE3D as:
\vspace{-0.2cm} 
\begin{equation}
\begin{split}
&\phi^{GeomE2D}(h,r,t)= \\
&(h_{0}\circ r_{0}+h_{1}\circ r_{1}+h_{2}\circ r_{2}-h_{12}\circ r_{12})\circ t_{0}-(h_{0}\circ r_{1}+h_{1}\circ r_{0}-h_{2}\circ r_{12}+h_{12}\circ r_{2})\circ t_{1}-\\
&(h_{0}\circ r_{2}+h_{2}\circ r_{0}+h_{1}\circ r_{12}-h_{12}\circ r_{1})\circ t_{2}+(h_{1}\circ r_{2}-h_{2}\circ r_{1}+h_{0}\circ r_{12}+h_{12}\circ r_{0})\circ t_{12}
\end{split}
\vspace{-0.1cm}
\label{GeomE2D}
\end{equation}

\vspace{-0.1cm} 
\begin{equation}
\begin{split}
&\phi^{GeomE3D}(h,r,t)=\\
&(h_{0}\circ r_{0}+h_{1}\circ r_{1}+h_{2}\circ r_{2}+h_{3}\circ r_{3}-h_{12}\circ r_{12}-h_{23}\circ r_{23}-h_{13}\circ r_{13}-h_{123}\circ r_{123})\circ t_{0}-\\
&(h_{0}\circ r_{1}+h_{1}\circ r_{0}-h_{2}\circ r_{12}+h_{12}\circ r_{2}-h_{3}\circ r_{13}+h_{13}\circ r_{3}-h_{23}\circ r_{123}-h_{123}\circ r_{23})\circ t_{1}-\\
&(h_{0}\circ r_{2}+h_{2}\circ r_{0}+h_{1}\circ r_{12}-h_{12}\circ r_{1}-h_{3}\circ r_{23}+h_{23}\circ r_{3}+h_{13}\circ r_{123}+h_{123}\circ r_{13})\circ t_{2}-\\
&(h_{0}\circ r_{3}+h_{3}\circ r_{0}+h_{1}\circ r_{13}-h_{13}\circ r_{1}+h_{2}\circ r_{23}-h_{23}\circ r_{2}-h_{12}\circ r_{123}-h_{123}\circ r_{12})\circ t_{3}+\\
&(h_{0}\circ r_{12}+h_{12}\circ r_{0}+h_{1}\circ r_{2}-h_{2}\circ r_{1}-h_{13}\circ r_{23}+h_{23}\circ r_{13}+h_{3}\circ r_{123}+h_{123}\circ r_{3})\circ t_{12}+\\
&(h_{0}\circ r_{23}+h_{23}\circ r_{0}+h_{1}\circ r_{123}+h_{123}\circ r_{1}+h_{2}\circ r_{3}-h_{3}\circ r_{2}-h_{12}\circ r_{13}+h_{13}\circ r_{12})\circ t_{23}+\\
&(h_{0}\circ r_{13}+h_{13}\circ r_{0}+h_{1}\circ r_{3}-h_{3}\circ r_{1}-h_{2}\circ r_{123}-h_{123}\circ r_{2}+h_{12}\circ r_{23}-h_{23}\circ r_{12})\circ t_{13}+\\
&(h_{0}\circ r_{123}+h_{123}\circ r_{0}+h_{1}\circ r_{23}+h_{23}\circ r_{1}-h_{2}\circ r_{13}-h_{13}\circ r_{2}+h_{3}\circ r_{12}+h_{12}\circ r_{3})\circ t_{123}\\
\end{split}
\label{GeomE3D}
\vspace{-0.1cm} 
\end{equation}
where $\circ$ denotes the Hadamard product.
\section{Proof of pRotatE assumption}~\label{proof pRotatE}
Apart from ComplEx and QuatE, GeomE also subsumes pRotatE. We start from the formulation of the scoring function of pRotatE and show that the scoring function is a special case of Equation~ \ref{Complex}. The scoring function of pRotatE is defined as
\begin{equation}
\begin{split}
    \phi^{pRotatE}(h,r,t) = -\| \mathbf{h}\circ \mathbf{r} - \mathbf{t}\|,
    \end{split}    \label{pRotatE}
\end{equation}
where the modulus of each element of relation vectors is $|\mathbf{r}_i| = 1, i=1,\dots,k,$ and $|\mathbf{h}_i| = |\mathbf{t}_i| = C \in \mathbb{R}^+.$
Therefore, we have
\begin{equation}
\begin{split}
    \phi^{pRotatE}(h,r,t) &= - \| \mathbf{h}\circ \mathbf{r} - \mathbf{t}\|= - \sqrt{\sum_{i=1}^{k} |\mathbf{h}_i \mathbf{r}_i - \mathbf{t}_i|^2} \\
    &= - \sqrt{\sum_{i=1}^{k} \big(|(\mathbf{h}_i \mathbf{r}_i)|^2 + |\mathbf{t}_i|^2 - 2 Re ((\mathbf{h}_i \mathbf{r}_i) \bar{\mathbf{t}}_i)\big)}.
    \end{split}
\end{equation}
Since $|\mathbf{r}_i| = 1$ and $|\mathbf{h}_i| = |\mathbf{t}_i| = C \in \mathbb{R}^+$, we have $\phi^{pRotatE}(h,r,t) = -\sqrt{2kC^2 + 2 Re ((\mathbf{h}_i \mathbf{r}_i) \bar{\mathbf{t}}_i)\big)}.$    Considering scalars in Equation~\ref{Complex}, i.e., $\mathbf{h}_{0}$, $\mathbf{r}_0$, $\mathbf{t}_0$, as real parts of complex values and bivectors $\mathbf{h}_{12}$, $\mathbf{r}_{12}$, $\mathbf{t}_{12}$ as imaginary parts of complex values, we can obtain $\phi^{GeomE2D}(h,r,t) = \frac{\phi^{pRotatE^2}(h,r,t)-2kC^2}{2}$.
Note that $2kC^2$ is a constant number as $k$ and $C$, and thus does not affect the overall ranking obtained by computing and sorting the scores of triples. For a triple $(h,r,t)$, there is a positive correlation between its GeomE score and pRotatE score since pRotatE scores are always non-positive. Therefore, GoemE2D and consequently GeomE3D \emph{subsumes} the pRotatE model in the terms of ranking.
\section{Proof of Modeling various Relation Patterns in a Matrix Form}~\label{proof in Matrix}
The geometric product between two 2-grade multivectors can also be represented in the form of matrix vector product as

\begin{equation}
    M_a \otimes_{2} M_b = Mat(M_a) \times vec(M_b) \times vec(e)^{T} = \begin{bmatrix}
a_0 & a_1 & a_2 & -a_{12} \\
a_1 & a_0 & a_{12} & -a_2 \\
a_2 & -a_{12} & a_0 & a_1\\
a_{12} & -a_2 & a_1 & a_0
\end{bmatrix} \times \begin{bmatrix}
b_0 \\
b_{1} \\
b_{2} \\
b_{12}
\end{bmatrix} \times
{\begin{bmatrix}
e_0 \\
e_{1} \\
e_{2} \\
e_{1}e_{2}
\end{bmatrix}}^{T},
\end{equation}
where $Mat(M_a)$ is a matrix corresponding to $M_a$, and $vec(M_b)$ is vector representation of $M_b$. Likewise, The coefficients of the geometric product of two 3-grade multivectors also can be represented as a multiplication of a $8\times8$ symmetric matrix and a vector.

Scoring function of GeomE can be written in the above form of matrix vector product,
\begin{equation}
\begin{split}
     \sum_{i}^{k}\textbf{Sc}(M_{h_i}\otimes_n M_{r_i} \otimes_n \overline{M_{t_i}}) =
     \sum_{i}^{k}\langle Mat(M_{r_i})\times vec(M_{h_i}) , vec(M_{t_i}) \odot \bar{\mathbf{1}} \rangle 
    %&\quad\quad\quad\ \ \quad\quad
    %h_{1}^{i},\cdots,h_{n}^{i}=0\\
    %    &\quad\quad\quad\ \ \quad\quad
    %t_{1}^{i},\cdots,t_{n}^{i}=0\\
\end{split}
\label{eq:matrixform}
\end{equation}
where $\times$ and $\odot$ denote matrix multiplication and element-wise vector multiplication.
$M_{h_{i}},M_{r_{i}},M_{t_{i}}\in \mathbb{G}^{n}$ are the $i$th multivector elements of $\mathbf{M}_{h},\mathbf{M}_{r},\mathbf{M}_{t}$, respectively.
% $h_{1}^{i},\cdots,h_{n}^{i}$ and $r_{1}^{i},\cdots,t_{n}^{i}$ represent the coefficents of vector parts of $M_{r_{i}}$.
$\bar{\mathbf{1}}$ is a $2^{n}$-dimensional vector used for changing the signs of coefficients of vector parts in an $n$-grade multivector ($n\leq 3$ in our case). 

For a triple $(h,r,t)$ where $r$ is involved in an (anti-)symmetry pattern, inversion pattern or composition pattern, we import the following constraints:
\begin{equation}
\begin{split}
Mat({M_{r_i}})\times vec(M_{h_i})=\lambda_{h_i}\cdot vec(M_{h_i})\\
 Mat({M_{r_i}})\times vec(M_{t_i})=\lambda_{t_i}\cdot vec(M_{t_i}).\\
\end{split}
\label{eq:constraints}
\end{equation}
where $\cdot$ denotes scalar multiplication, $\lambda_{h_i}$ and $\lambda_{t_i}$ are the eigenvalues corresponding to $vec(M_{h_i})$ and $vec(M_{t_i})$.

% Under the third and fourth constraints in Equation~\ref{eq:constraints}, we have $\textbf{Sc}(M_{h_i}\otimes_{n} M_{r_i} \otimes_{n} \overline{M_{t_i}})=\langle Mat(M_{r_i})\times vec(M_{h_i}), vec(M_{t_i})\rangle$ and $\textbf{Sc}(M_{h_i}\otimes_{n} M_{r_i} \otimes_{n} \overline{M_{t_i}})=\langle Mat(M_{r_i})\times vec(M_{t_i}), vec(M_{h_i})\rangle$

\textbf{(Anti-)Symmetry}
By utilizing the conjugation of embeddings of tail entities, our framework can model both two patterns.
Concretely, considering equation~\ref{eq:matrixform} and~\ref{eq:constraints}, we show GeomE models symmetric pattern by $\phi(h,r,t) - \phi(t,r,h) = 0$ as follows
\begin{equation}
\begin{split}
     &\textbf{Sc}(M_{h_i}\otimes_n M_{r_i} \otimes_n \overline{M_{t_i}})  - \textbf{Sc}(M_{t_i}\otimes_n M_{r_i} \otimes_n \overline{M_{h_i}}) =\\
    &\langle Mat(M_{r_i})\times vec(M_{h_i}) , vec(M_{t_i}) \odot \bar{\mathbf{1}} \rangle -  \langle Mat(M_{r_i})\times vec(M_{t_i}) , vec(M_{h_i}) \odot \bar{\mathbf{1}} \rangle = \\
    &\langle \lambda_{hi}\cdot vec(M_{h_i}) , vec(M_{t_i}) \odot \bar{\mathbf{1}} \rangle -  \langle \lambda_{ti}\cdot vec(M_{t_i}) , vec(M_{h_i}) \odot \bar{\mathbf{1}} \rangle =\\
    &\lambda_{hi} \cdot\langle vec(M_{h_i}) , vec(M_{t_i}) \odot \bar{\mathbf{1}} \rangle -  \lambda_{ti}\cdot \langle vec(M_{t_i}) , vec(M_{h_i}) \odot \bar{\mathbf{1}} \rangle.
\end{split}
\end{equation}

Let assume that the matrix $Mat(M_{r_i})$ is householder. Therefore, it has two eigenvalues $\{-1,1\}$. The eigenvectors corresponding to -1 are orthogonal to the eigenvalues corresponding to 1. 
There are two conditions
\begin{itemize}
    \item Both of $vec(M_{t_i}) , vec(M_{h_i}) $ are eigenvectors (parallel) corresponding to the same eigenvalue. Therefore, we have 
    
\begin{equation}
\begin{split}
    &\lambda_{hi} \langle vec(M_{h_i}) , vec(M_{t_i}) \odot \bar{\mathbf{1}} \rangle -  \lambda_{ti} \langle vec(M_{t_i}) , vec(M_{h_i}) \odot \bar{\mathbf{1}} \rangle = \\
    & \langle vec(M_{h_i}) , vec(M_{t_i}) \odot \bar{\mathbf{1}} \rangle -  \langle vec(M_{t_i}) , vec(M_{h_i}) \odot \bar{\mathbf{1}} \rangle = \\
    &\langle vec(M_{h_i}) , vec(M_{t_i}) \odot \bar{\mathbf{1}} \rangle -  \langle vec(M_{h_i}) , vec(M_{t_i}) \odot \bar{\mathbf{1}} \rangle = 0.
\end{split}
\end{equation}
\item  Both of $vec(M_{t_i}) , vec(M_{h_i}) $ are eignevectors (orthogonal) corresponding to different eigenvalues. Therefore, we have 
    
\begin{equation}
\begin{split}
    &\lambda_{hi} \langle vec(M_{h_i}) , vec(M_{t_i}) \odot \bar{\mathbf{1}} \rangle -  \lambda_{ti} \langle vec(M_{t_i}) , vec(M_{h_i}) \odot \bar{\mathbf{1}} \rangle = \\
    & \langle vec(M_{h_i}) , vec(M_{t_i}) \odot \bar{\mathbf{1}} \rangle +  \langle vec(M_{t_i}) , vec(M_{h_i}) \odot \bar{\mathbf{1}} \rangle = \\
    &\langle vec(M_{h_i}) , vec(M_{t_i}) \odot \bar{\mathbf{1}} \rangle =  2 \langle vec(M_{h_i}) , vec(M_{t_i}) \odot \bar{\mathbf{1}} \rangle.
\end{split}
\end{equation}
The abovementioned equation equals to zero if for either $vec(M_{h_i})$ or $vec(M_{t_i})$, the elements (coefficents of vector parts in this case) corresponding to the negative sign (-1) of $\bar{\mathbf{1}}$ will be zero. 
\end{itemize}
The abovementioned conditions hold for each multivector element $M_{i}$ of the k-dimensional embeddings $\mathbf{M}$, i.e.~$i = 1, \ldots, k$. Therefore, there are $2^k$ possible options (capacity of model) to have $\phi(h,r,t) - \phi(t,r,h) = 0$ (modeling symmetric pattern).

\textbf{Inversion} 
Given two relations $r_1, r_2$ which form inverse pattern i.e.~$r_1 = r^{-1}_2$ (e.g.~$r_1 = $\textit{SonOf}, $r_2 =$\textit{FatherOf}), we show that GeomE models inverse pattern by $\phi(h,r_1,t) - \phi(t,r_2,h) = 0$. This is proved as follows

\begin{equation}
\begin{split}
     &\textbf{Sc}(M_{h_i}\otimes_n M_{r_{1i}} \otimes_n \overline{M_{t_i}})  - \textbf{Sc}(M_{t_i}\otimes_n M_{r_{2i}} \otimes_n \overline{M_{h_i}}) =\\
    &\langle Mat(M_{r_{1i}})\times vec(M_{h_i}) , vec(M_{t_i}) \odot \bar{\mathbf{1}} \rangle -  \langle Mat(M_{r_{2i}})\times vec(M_{t_i}) , vec(M_{h_i}) \odot \bar{\mathbf{1}} \rangle = \\
    &\langle \lambda_{1hi}\cdot vec(M_{h_i}) , vec(M_{t_i}) \odot \bar{\mathbf{1}} \rangle -  \langle \lambda_{2ti}\cdot vec(M_{t_i}) , vec(M_{h_i}) \odot \bar{\mathbf{1}} \rangle =\\
    &\lambda_{1hi} \cdot\langle vec(M_{h_i}) , vec(M_{t_i}) \odot \bar{\mathbf{1}} \rangle -  \lambda_{2ti}\cdot \langle vec(M_{t_i}) , vec(M_{h_i}) \odot \bar{\mathbf{1}} \rangle.
\end{split}
\label{eq:inverse}
\end{equation}

Let assume that the matrices of $Mat(M_{r_{1i}})$ and $Mat(M_{r_{2i}})$ have same eigenvalues $\lambda_{1i} = \lambda_{2i}$. Therefore, we have

\begin{equation}
\begin{split}
    &\lambda_{1hi} \langle vec(M_{h_i}) , vec(M_{t_i}) \odot \bar{\mathbf{1}} \rangle -  \lambda_{2ti} \langle vec(M_{t_i}) , vec(M_{h_i}) \odot \bar{\mathbf{1}} \rangle = \\
    & \lambda_{1hi} (\langle vec(M_{h_i}) , vec(M_{t_i}) \odot \bar{\mathbf{1}} \rangle -  \langle vec(M_{t_i}) , vec(M_{h_i}) \odot \bar{\mathbf{1}} \rangle) = \\
    &\lambda_{1hi} (\langle vec(M_{h_i}) , vec(M_{t_i}) \odot \bar{\mathbf{1}} \rangle -  \langle vec(M_{h_i}) , vec(M_{t_i}) \odot \bar{\mathbf{1}} \rangle) = 0.
\end{split}
\end{equation}

Since for $n$-grade multivector, there are $2^n$ variables in the vector, the corrsponding matrices $Mat(M_{r_{1i}}), Mat(M_{r_{2i}})$ are $2^n \times 2^n$ dimensional. 
Since a $2^n \times 2^n$ matrix has at most $2^n$ distinct eigenvalues/eigenvectors, GeomE with $k$ dimension for embedding can at most represent $2^{n^k}$ distinct entity embedding vectors (model capacity) for encoding inverse pattern.

\textbf{Composition} 
By enforcing the coefficents of vector parts of $\mathbf{M}_h$ and $\mathbf{M}_t$ to be zero, we obtain
\begin{equation}
\begin{split}
&\textbf{Sc}(M_{h_i}\otimes_n M_{r_i} \otimes_n \overline{M_{t_i}}) = \langle Mat(M_{r_i})\times vec(M_{h_i}) , vec(M_{t_i}) \rangle\\
&\text{subject to:} 
 \quad
    h_{1}^{i},\cdots,h_{n}^{i}=0\\
        &\quad\quad\quad\ \ \quad\quad
    t_{1}^{i},\cdots,t_{n}^{i}=0\\
\end{split}
\label{eq:transform of Sc}
\end{equation}
where $h_{1}^{i},\cdots,h_{n}^{i}$ and $t_{1}^{i},\cdots,t_{n}^{i}$ are the vector parts of $M_{h_i}$ and $M_{t_i}$, $n\leq 3$ in our case.

Since $vec(M_{h_{i}})$ and $vec(M_{t_{i}})$ are eigenvectors of $Mat(M_{r_{i}})$ (defined in Equation~\ref{eq:constraints}), the maximization of $ \textbf{Sc}(M_{h_{i}}\otimes_{n} M_{r_{i}} \otimes_{n} \overline{M_{t_i}})$ is equivalent to minimizing $\angle(Mat(M_{r_{i}})\times vec(M_{h_{i}}) , vec(M_{t_{i}}))$ under the following constraints,
\begin{equation}
\begin{split}
    &\text{arg}\ \text{max}\ \textbf{Sc}(M_{h_i}\otimes_n M_{r_i} \otimes_n \overline{M_{t_i}}) =
    \text{arg}\ \text{max}\ \langle Mat(M_{r_i})\times vec(M_{h_i}) , vec(M_{t_i}) \rangle = \\
    &\text{arg}\ \text{min}\ \angle(Mat(M_{r_i})\times vec(M_{h_i}) , vec(M_{t_i}))\\
    &\text{subject to:} \quad Mat({M_{r_i}})\times vec(M_{h_i})=\lambda_{h_i}\cdot vec(M_{h_i})\\
    &\quad\quad\quad\ \ \quad\quad Mat({M_{r_i}})\times vec(M_{t_i})=\lambda_{t_i}\cdot vec(M_{t_i}).\\
    &\quad\quad\quad\ \ \quad\quad
    h_{1}^{i},\cdots,h_{n}^{i}=0\\
        &\quad\quad\quad\ \ \quad\quad
    t_{1}^{i},\cdots,t_{n}^{i}=0\\
\end{split}
\label{eq:optimization}
\end{equation}

Note that eigenvectors are scale-free. It means given $A\times x=\lambda\cdot x$ where $A$ is a matrix, $x$ and $\lambda$ are its eigenvector and the corresponding eigenvalue, the multiplication of $\lambda$ by any real number $c$ is also an eigenvector, i.e., $A\times(c\cdot x)=\lambda \cdot c\cdot x$. Therefore, maximization of $\langle Mat(M_{r_i})\times vec(M_{h_i}) , vec(M_{t_i}) \rangle$, is equivalent to minimizing the angle between two vectors under the scale-free condition. Based on the above-mentioned assumption, and in order to model composition pattern $r_1(h,o) \land r_2(o , t) \Rightarrow r_3(h, t)$, we have
\begin{equation}
    \begin{split}
        Mat(M_{r1i})\times vec(M_{hi}) = \alpha_1 \cdot vec(M_{oi}), \\
        Mat(M_{r2i})\times vec(M_{oi}) = \alpha_2 \cdot vec(M_{ti}), \\
        Mat(M_{r3i})\times vec(M_{hi}) = \alpha_3 \cdot vec(M_{ti}), \\
    \end{split}
\end{equation}
where $\alpha_{1},\alpha_{2},\alpha_{3}$ are real numbers. Furthermore, we obtain the following connection between embeddings of $r_1$, $r_2$ and $r_3$.
\begin{equation}
    \begin{split}
 Mat(M_{r_3i}) =\alpha \cdot  Mat(M_{r_1i}) \times Mat(M_{r_2i})
    \end{split}
    \label{eq:relconstraint}
\end{equation}
where $\alpha=\alpha_{3}/(\alpha_{1}\cdot \alpha_{2})$ can be any real number. Thus, $\forall h,o,t\ \  r_1(h,o) \land r_2(o , t) \Rightarrow r_3(h, t)$ holds true under the constraints in Equation~\ref{eq:constraints} when Equation~\ref{eq:relconstraint} is valid.

\section{Dataset}~\label{datasets}
\begin{table}[h]
\begin{center}
\resizebox{0.8\textwidth}{!}{
\begin{tabular}{|c|ccccc|}
\hline  Datasets & \#Entities & \#Relations &  \#Training&  \#Validation&  \#Training\\ \hline
FB15K&14951& 1,345&483,142& 50,000& 59,071\\
WN18&40,943&18& 141,442& 5,000& 5,000\\
FB15K-237&14,541& 237& 272,115& 17,535& 20,466\\
WN18RR&40,943&11 &86,835& 3,034& 3,134\\
\hline
\end{tabular}}
\end{center}
\caption{ Number of entities, relations, and observed triples in each split for four benchmarks.}
\vspace{-0.3cm}
\label{statics}
\end{table}
\begin{table}[h]
\begin{center}
\resizebox{0.8\textwidth}{!}{
\begin{tabular}{cccc}
\hline  Model & Scoreing Function & Relation Parameters &  $\mathcal{O}_{space}$\\ \hline
\specialrule{0em}{1pt}{1pt}
RESCAL&$-||\mathbf{h}^{\top}\mathbf{W_{r}\mathbf{t}}||$&$\mathbf{W_{r}}\in \mathbb{R}^{k^2}$&$\mathcal{O}(n_{e}k+n_{r}k^2)$\\
DistMult&$<\mathbf{h,r,t}>$&$\mathbf{r}\in \mathbb{R}^{k}$&$\mathcal{O}(n_{e}k+n_{r}k)$\\
ComplEx&\textbf{Re}$(\mathbf{<h,r,\overline{t}>})$&$\mathbf{r}\in \mathbb{C}^{k}$&$\mathcal{O}(n_{e}k+n_{r}k)$\\
ConvE&$f(\text{vec}(f([\mathbf{W_{h};W_{r}}]\ast\boldsymbol{\mathcal{\omega}}))\textbf{W})\mathbf{t}$&$\mathbf{W_{r}}\in\mathbb{R}^{k}$&$\mathcal{O}(n_{e}k+n_{r}k)$\\
(p)RotatE&$-||\mathbf{h\circ r-t}||$&$\mathbf{r}\in \mathbb{C}^{k}$&$\mathcal{O}(n_{e}k+n_{r}k)$\\\
QuatE&$\mathbf{Q_{h}\otimes W_{r}^{\triangleleft}\cdot Q_{t}}$&$\mathbf{W_{r}}\in\mathbb{H}^{k}$&$\mathcal{O}(n_{e}k+n_{r}k)$\\
\hline
\specialrule{0em}{1pt}{1pt}
GeomE2D&$\langle \textbf{Sc}(\textbf{M}_{h}\otimes_2 \textbf{M}_{r} \otimes_2 \overline{\textbf{M}_{t}}),{\textbf{1}}\rangle$&$\mathbf{M_{r}}\in\mathbb{G}^{2\times k}$&$\mathcal{O}(n_{e}k+n_{r}k)$\\
GeomE3D&$\langle \textbf{Sc}(\textbf{M}_{h}\otimes_3 \textbf{M}_{r} \otimes_3 \overline{\textbf{M}_{t}}),{\textbf{1}}\rangle$&$\mathbf{M_{r}}\in\mathbb{G}^{3\times k}$&$\mathcal{O}(n_{e}k+n_{r}k)$\\

\hline
\end{tabular}}
\end{center}
\caption{Scoring functions of state-of-the-art link prediction models, their parameters as well as their time complexity and space complexity. $\text{vec}()$ denotes the matrix flattening. $\ast$ denotes the convolution operator. $f$ denotes a non-linear function. $\otimes$ denotes the Hamilton product. $\mathbb{H}$ denotes a hypercomplex space. ${\triangleleft}$ denotes the normalization of quaternions.}\label{complexity}
\vspace{-0.3cm}
\end{table}
\end{appendices}
